# Supplementary material for: Maximum Flow and Minimum-Cost Flow in Almost-Linear Time
Source: arXiv:2203.00671 source file (2022-04-22)
Supplement: Supplementary file 1 [file spanner_appendix.tex]

\section{Expander Proofs}
\label{app:expanderStatement}
